# Supplementary material for: LoHoRavens: A Long-Horizon Language-Conditioned Benchmark for Robotic Tabletop Manipulation
Source: arXiv:2310.12020 source file (2023-10-23)
Supplement: Supplementary file 1 [file appendix.tex]

\section*{APPENDIX}

% Appendixes should appear before the acknowledgment.

\subsection{Task details}
\label{task_details}
%\todo{Please follow the Appendix B of~\cite{jiang2023vima} to write the following explanations of each task. Note for all the size reasoning tasks, there are only 2 sizes which are described as ``smaller" and ``bigger".}
% \todo{Please follow the appendix of to write the following explanations of each task.}

\subsubsection{\textbf{Primitive Pick-And-Place Task}} This task asks the robot to pick up a block of a specific color or size and place it at a relative or absolute position.

%(four types: pick up the blue block and place it on the yellow block; pick up the smaller/bigger blue block and place it on the smaller/bigger yellow block; pick up the blue block and place it on the left on the yellow block; pick up the blue block and place it on the center of the table.)

\paragraph{Instruction} Pick up the \texttt{[SIZE?/COLOR]} block and place it \texttt{[POSITION]} the \texttt{[SIZE?/COLOR]} block; Pick up the \texttt{[SIZE?/COLOR]} block and place it \texttt{[POSITION]} of the table. 
\paragraph{Variables} SIZE=[smaller,bigger], COLOR=[blue, yellow, red, green, pink, grey, white], POSITION=[on, on the left of, on the right of, in the center of, above, below]
\paragraph{Description} The task requires spatial reasoning and the ability to discern colors and shapes. The task is a simple pick up block and place block, but the color of the source and target blocks can be varied as well as their sizes. Target position can either be relative (e.g. left of the green block) or absolute (e.g. at the center of the table).
\paragraph{Capabilities} Reasoning about colors, shapes, sizes and spatial relations.
\paragraph{Success criteria} All specified blocks are placed in the specified areas.

\subsubsection{\textbf{Put all the blocks in the bowls with matching colors}}
This task requires the robot to correctly match and place blocks of specific colors into corresponding bowls.

\paragraph{Instruction} Place all blocks into bowls of the respective color, e.g. blue block in blue bowl and so on.

\paragraph{Variables} -

\paragraph{Description} In this task, there are several colored blocks and matching colored bowls. The robot needs to correctly identify the color of each block and place it into the bowl with the corresponding color. For example, the blue block should go into the blue bowl, the yellow block into the yellow bowl, and so on.

\paragraph{Capabilities} Color recognition.

\paragraph{Success criteria} All blocks are placed in the bowls with matching colors.

\subsubsection{\textbf{Put all the blocks in the bowls with mismatching colors}}
This task requires the robot to intentionally mismatch blocks with bowls of different colors.

\paragraph{Instruction} Place all blocks into the  bowls of different color.

\paragraph{Variables} -

\paragraph{Description} In this task, the robot must place blocks into bowls with colors that do not match. Each block has a specific color, and there are bowls with mismatched colors. For example, the robot should place a blue block into a yellow bowl, a red block into a green bowl, and so on.

\paragraph{Capabilities} Color recognition.

\paragraph{Success criteria} All blocks are placed in bowls with colors that do not match the blocks' colors.

\subsubsection{\textbf{Stack blocks of the same size}}
This task requires the robot to stack blocks of identical sizes on top of each other.

\paragraph{Instruction} Stack the \texttt{[SIZE]} blocks on top of each other.

\paragraph{Variables} SIZE=[smaller, bigger]

\paragraph{Description} In this task, there are blocks of different sizes available, and the robot must identify blocks of the same size and stack them on top of each other. For example, if there are two smaller blocks and three bigger blocks, the robot should create two stacks, one with the smaller blocks and one with the bigger blocks.

\paragraph{Capabilities} Size recognition..

\paragraph{Success criteria} All blocks are stacked according to their size, with blocks of the same size stacked together.

\subsubsection{\textbf{Stack smaller blocks over bigger blocks of the same color}}
This task requires the robot to stack blocks of the same color with smaller blocks on top of bigger blocks.

\paragraph{Instruction} Stack the \texttt{[COLOR]} blocks with smaller sizes on top of the \texttt{[COLOR]} blocks with bigger sizes.

\paragraph{Variables} COLOR=[blue, yellow, red, green, pink, grey, white]

\paragraph{Description} In this task, there are blocks of different colors and sizes available, and the robot must identify blocks of the same color and stack them with smaller blocks on top of bigger blocks. For example, if there are two blue blocks (one smaller and one bigger), the robot should stack the smaller blue block on top of the bigger blue block. This applies to blocks of all colors.

\paragraph{Capabilities} Color recognition, size recognition.

\paragraph{Success criteria} All blocks of the same color are stacked correctly, with smaller blocks on top of bigger blocks.

\subsubsection{\textbf{Stack blocks in alternate colors}}
This task requires the robot to stack blocks in an alternating color pattern.

\paragraph{Instruction} Stack the blocks in an alternate color pattern.

\paragraph{Variables} -

\paragraph{Description} In this task, there are blocks of various colors available, and the robot must stack them in a pattern where colors alternate. For example, if there are blue, yellow, and red blocks, the robot should stack them as: blue, yellow, red, blue, yellow, red, and so on.

\paragraph{Capabilities} Color recognition.

\paragraph{Success criteria} The blocks are stacked in an alternating color pattern.

\subsubsection{\textbf{Stack blocks of the same color in the zone with the same color, with the bigger blocks underneath}}
This task requires the robot to stack blocks of the same color in designated zones, with bigger blocks at the bottom.

\paragraph{Instruction} Stack the \texttt{[COLOR]} blocks in the \texttt{[COLOR]} zone, with the bigger blocks at the bottom.

\paragraph{Variables} COLOR=[blue, yellow, red, green, pink, grey, white]

\paragraph{Description} In this task, there are blocks of different colors and sizes available. The robot must identify blocks of the same color and stack them in a specified zone with the bigger blocks placed at the bottom. For example, if there are two red blocks (one bigger and one smaller), the robot should stack the smaller red block on top of the bigger red block in the designated red zone.

\paragraph{Capabilities} Color recognition, size recognition.

\paragraph{Success criteria} Blocks of the same color are stacked correctly in their designated zones, with bigger blocks at the bottom.

\subsubsection{\textbf{Move all the blocks in the top right zone to the bottom left zone}}
This task requires the robot to relocate blocks from the top right zone to the bottom left zone.

\paragraph{Instruction} Move all the blocks in the top right zone to the bottom left zone.

\paragraph{Variables} -

\paragraph{Description} In this task, there are two zones, a top right zone and a bottom left zone, each containing blocks. The robot's objective is to move all the blocks from the top right zone to the bottom left zone.

\paragraph{Capabilities} Spatial reasoning.

\paragraph{Success criteria} All blocks from the top right zone are successfully moved to the bottom left zone.

\subsubsection{\textbf{Stack all blocks that occur in even numbers (there are only two colors)}}
This task requires the robot to stack blocks with even-numbered occurrence, considering there are only two colors of blocks.

\paragraph{Instruction} Stack all the blocks that occur in even numbers.

\paragraph{Variables} -

\paragraph{Description} In this task, there are two colors of blocks available, and the robot must stack blocks that occur in even numbers.

\paragraph{Capabilities} Counting.

\paragraph{Success criteria} All blocks that occur in even numbers are successfully stacked.

\subsubsection{\textbf{Let all the blocks form a straight line}}
This task requires the robot to arrange all the blocks in a straight line.

\paragraph{Instruction} Arrange all the blocks in a straight line.

\paragraph{Variables} -

\paragraph{Description} In this task, there are multiple blocks, and the robot must arrange them in a straight line, with each block positioned adjacent to the next one.

\paragraph{Capabilities} Spatial reasoning.

\paragraph{Success criteria} All blocks are arranged in a straight line.

\subsubsection{\textbf{Stack blocks of the same color, given there are multiple blocks with the same color}}
This task requires the robot to stack blocks of the same color when there are multiple blocks with the same color available.

\paragraph{Instruction} Stack the blocks of the same \texttt{[COLOR]} color on top of each other.

\paragraph{Variables} COLOR=[blue, yellow, red, green, pink, grey, white]

\paragraph{Description} In this task, there are blocks of different colors, and some colors have multiple blocks available. The robot must identify blocks of the same color and stack them on top of each other. For example, if there are three red blocks, the robot should stack all the red blocks on top of each other.

\paragraph{Capabilities} Color recognition.

\paragraph{Success criteria} Blocks of the same color are stacked correctly on top of each other.

\paragraph{Capabilities} Reference resolution

\subsection{Prompts for LLMs and VLMs}
